# Supplementary material for: Automated Evaluation of One-Loop Six-Point Processes for the LHC
Source: arXiv:0903.0947 source file (2009-03-05)
Supplement: Supplementary file 1 [file appendix-software.tex]

In this section I give an overview over the software I used for my
calculations. 
\begin{description}
\item[\form] is a Symbolic Manipulation System
specialised to handle extremely large expressions of
many millions of terms in an efficient way.
\\See~\cite{Vermaseren:2000nd,Vermaseren:2006ag}
and~\url{http://www.nikhef.nl/~form/}.
\item[\qgraf] is a computer program for automatic
generation of \person{Feynman} diagrams in field theories.
\\See~\cite{Nogueira:1991ex}
and~\url{http://cfif.ist.utl.pt/~paulo/qgraf.html}.
\item[\maple] is a general purpose Computer Algebra System.
\maple is a registered trademark of Waterloo Maple Inc.
\\See~\url{http://www.maplesoft.com}
\end{description}
