# Supplementary material for: Automated Evaluation of One-Loop Six-Point Processes for the LHC
Source: arXiv:0903.0947 source file (2009-03-05)
Supplement: Supplementary file 2 [file appendix-wigner.tex]

\chapter{\texorpdfstring{$\mathrm{SU}(N)$}{SU(N)} \person{Wigner} Coefficients}
\label{app:appendix-wigner}
This appendix gives a list of \person{Wigner} coefficients that appear in
amplitude calculations when the colour algebra is carried out using recoupling
relations. It should be noted that only on representative diagram is given for
each topology. All coefficients are given for the choice~$T_R=1/2$.
\begin{fmffile}{qcd-wigner}
\begin{subequations}
\begin{align}
% qqqggg
\parbox[c][\height+1.5\baselineskip][c]{20mm}{%nl
\begin{fmfchar*}(20,20)
\fmfsurround{v1,v2,v3}
\fmfdot{v1,v2,v3,z}
\fmf{fermion,right=0.5}{v1,v2}
\fmf{fermion,right=0.5}{v2,v3}
\fmf{fermion,right=0.5}{v3,v1}
\fmf{dashes}{v1,z}
\fmf{dashes}{v2,z}
\fmf{dashes}{v3,z}
\end{fmfchar*}}&\quad=-\frac14N_C(N_C^2-1)\displaybreak[1]\\
% qqqqgg
\parbox[c][\height+1.5\baselineskip][c]{20mm}{%nl
\begin{fmfchar*}(20,20)
\fmfsurround{v1,v2,v3}
\fmfdot{v1,v2,v3,z}
\fmf{fermion,right=0.5}{v1,v2}
\fmf{fermion,right=0.5}{v2,v3}
\fmf{dashes,right=0.5}{v3,v1}
\fmf{fermion}{z,v1}
\fmf{dashes}{v2,z}
\fmf{fermion}{v3,z}
\end{fmfchar*}}&\quad=-\frac14\frac{N_C^2-1}{N_C}\displaybreak[1]\\
% gggggg
\parbox[c][\height+1.5\baselineskip][c]{20mm}{%nl
\begin{fmfchar*}(20,20)
\fmfsurround{v1,v2,v3}
\fmfdot{v1,v2,v3,z}
\fmf{dashes,right=0.5}{v1,v2}
\fmf{dashes,right=0.5}{v2,v3}
\fmf{dashes,right=0.5}{v3,v1}
\fmf{dashes}{z,v1}
\fmf{dashes}{v2,z}
\fmf{dashes}{v3,z}
\end{fmfchar*}}&\quad=\frac12N_C^2(N_C^2-1)\displaybreak[1]\\
% qqqggs
\parbox[c][\height+1.5\baselineskip][c]{20mm}{%nl
\begin{fmfchar*}(20,20)
\fmfsurround{v1,v2,v3}
\fmfdot{v1,v2,v3,z}
\fmf{fermion,right=0.5}{v1,v2}
\fmf{fermion,right=0.5}{v2,v3}
\fmf{fermion,right=0.5}{v3,v1}
\fmf{dots}{v1,z}
\fmf{dashes}{v2,z}
\fmf{dashes}{v3,z}
\end{fmfchar*}}&\quad=\quad
% qqqqgs
\parbox[c][\height+1.5\baselineskip][c]{20mm}{%nl
\begin{fmfchar*}(20,20)
\fmfsurround{v1,v2,v3}
\fmfdot{v1,v2,v3,z}
\fmf{fermion,right=0.5}{v1,v2}
\fmf{fermion,right=0.5}{v2,v3}
\fmf{dashes,right=0.5}{v3,v1}
\fmf{fermion}{z,v1}
\fmf{dots}{v2,z}
\fmf{fermion}{v3,z}
\end{fmfchar*}}\quad=\quad
% qqg
\parbox[c][\height+0.3\baselineskip][c]{10mm}{%nl
\begin{fmfchar*}(10,10)
\fmfleft{p}\fmfright{q}
\fmfdot{p,q}
\fmf{fermion,left}{p,q,p}
\fmf{dashes}{p,q}
\end{fmfchar*}}\quad=\frac12(N_C^2-1)\displaybreak[1]\\
% gggggs
\parbox[c][\height+1.5\baselineskip][c]{20mm}{%nl
\begin{fmfchar*}(20,20)
\fmfsurround{v1,v2,v3}
\fmfdot{v1,v2,v3,z}
\fmf{dashes,right=0.5}{v1,v2}
\fmf{dashes,right=0.5}{v2,v3}
\fmf{dashes,right=0.5}{v3,v1}
\fmf{dots}{z,v1}
\fmf{dashes}{v2,z}
\fmf{dashes}{v3,z}
\end{fmfchar*}}&\quad=\quad
% ggg
\parbox[c][\height+0.3\baselineskip][c]{10mm}{%nl
\begin{fmfchar*}(10,10)
\fmfleft{p}\fmfright{q}
\fmfdot{p,q}
\fmf{dashes,left}{p,q,p}
\fmf{dashes}{p,q}
\end{fmfchar*}}\quad=N_C(N_C^2-1)\displaybreak[1]\\
% ggs
\parbox[c][\height+0.3\baselineskip][c]{10mm}{%nl
\begin{fmfchar*}(10,10)
\fmfleft{p}\fmfright{q}
\fmfdot{p,q}
\fmf{dashes,left}{p,q,p}
\fmf{dots}{p,q}
\end{fmfchar*}}&\quad=\quad
% gg
\parbox[c][\height+0.3\baselineskip][c]{10mm}{%nl
\begin{fmfchar*}(10,10)
\fmfleft{p}\fmfright{q}
\fmf{dashes,left}{p,q,p}
\end{fmfchar*}}\quad=\quad
N_C^2-1\displaybreak[1]\\
% qqs
\parbox[c][\height+0.3\baselineskip][c]{10mm}{%nl
\begin{fmfchar*}(10,10)
\fmfleft{p}\fmfright{q}
\fmfdot{p,q}
\fmf{fermion,left}{p,q,p}
\fmf{dots}{p,q}
\end{fmfchar*}}&\quad=\quad
% qq
\parbox[c][\height+0.3\baselineskip][c]{10mm}{%nl
\begin{fmfchar*}(10,10)
\fmfleft{p}\fmfright{q}
\fmf{fermion,left}{p,q,p}
\end{fmfchar*}}\quad=\quad
N_C
\end{align}
\end{subequations}
\end{fmffile}
